# Supplementary material for: HAGNN: Hybrid Aggregation for Heterogeneous Graph Neural Networks
Source: arXiv:2307.01636 source file (2024-12-15)
Supplement: Supplementary file 1 [file sec7-supplementary.tex]

\appendix

\subsection{Implementations and Configurations of Baselines}
\label{ss:conf}
We use the HGB benchmark to evaluate the performance of all baselines. 
In HGB, implementations of baselines are based on their official codes to avoid errors introduced by re-implementation.
Next, we present the configurations of baselines in the node classification and link prediction tasks, respectively.
For brevity, we denote the dimension of node embedding as $d$, the dimension of edge embedding as $d_e$, the dimension of attention vector (if exists) as $d_a$, the number of GNN layers as $L$, the number of attention heads as $n_h$, the negative slope of LeakyReLU as $s$.
\subsubsection{Node Classification}
The baselines in the node classification task contain HAN, GTN, HetSANN, MAGNN, HGT, HetGNN, GCN, GAT, SimpleHGN, HGNN-AC, BPHGNN, AMHGNN, and HINormer.
\begin{itemize}
\item \emph{HAN:}  $d=8$, $d_a=128$, $n_h=8$, and $L=2$.
% For the input feature type, we use $feat=2$ in Freebase, and $feat=1$ in other datasets. 
%We have also tried larger $d$, but the variation of performance becomes very large. Therefore, We keep $d=8$ as suggested in HAN's code.
\item \emph{GTN:} The adaptive learning rate is employed for all datasets. $d=64$ and the number of GTN channels is 2. For DBLP and ACM,  $L=2$. For IMDB,  $L=3$. 
\item \emph{HetSANN:} For ACM, $d=64$, $L=3$, and $n_h=8$. For IMDB, $d=32$, $L=2$, and $n_h=4$. For DBLP, $d=64$, $L=2$, and $n_h=4$.
\item \emph{MAGNN:} For DBLP and ACM, the batch size is 8, and the number of neighbor samples is 100. For IMDB, we use full batch training.
\item \emph{HGT:} We use the layer normalization in each layer, and set $d=64$ and $n_h=8$ for all datasets. $L$ is set to 2, 3, 5 for ACM, DBLP and IMDB, respectively.
\item \emph{HetGNN:} $d=128$, and the batch size is 200 for all datasets. For random walk, we set the walk length to 30 and the window size to 5.
\item \emph{GCN:} $d=64$. $L=3$ for DBLP and ACM, and $L=4$ for IMDB. 
\item \emph{GAT:} $d=64$ and $n_h=8$ for all datasets. For DBLP and ACM, $s=0.05$ and $L=3$. For IMDB, we set $s=0.1$ and $L=5$. 
% \item \emph{RGCN:} We set $L=5$ for all datasets. For ACM, we set $d=16$. For DBLP and Freebase, we set $d=16$. For IMDB, we set $d=32$.
\item \emph{SimpleHGN:}  $d=d_e=64$, $n_h=8$, and the edge residual $\beta=0.05$ for all datasets. For DBLP and ACM, we set $L=3$ and $s=0.05$. For IMDB, we set $L=6$ and $s=0.1$. 
\item \emph{HGNN-AC:}  $d=64$, $n_h=8$, the divided ratio $\alpha$ of $N^+$ is 0.3, and the loss weighted coefficient $\lambda$ is 0.5 for all datasets.
\item \emph{BPHGNN:} $d=64$, $n_h=8$, the number of aggregation layers is 2, and the tunable temperature hyperparameter $\tau$ is 0.1. For the node classification task, the hyperparameter for tuning the importance of contrastive learning $\gamma$ is 0.01.
\item \emph{AMHGNN:}  $d=64$. $r=1.0$, $\theta=0.0001$, $\theta_{env}=0.83$ for DBLP, $r=1.3$, $\theta=0.7$, $\theta_{env}=0.3$ for ACM. $\theta$ and $\theta_{env}$ are used for Markov calculation.
\item \emph{HINormer:} The range of sequence length S is [10, 200], the hidden dimension $d$ is set to 256 and the number of head $n_h$ is set to 2
for all datasets. The number of layers for local structure encoder $K_s$ and heterogeneous relation encoder $K_h$ is set to 5 for DBLP, 4 for IMDB and 3 for others.
\end{itemize}

\subsubsection{Link prediction}
The baselines in the link prediction task contain GATNE, HetGNN, GCN, GAT, SimpleHGN, and AutoAC.
\begin{itemize}
  
    \item \emph{GATNE:} $d=200$, $d_e=10$, and $d_a=20$ for all datasets.
    For the random walk, we set the walk length to 30 and the window size to 5. For neighbor sampling, we set the number of negative samples for optimization to 5 and the number of neighbor samples for aggregation to 10.
    \item \emph{HetGNN:} $d=128$, and the batch size is 200 for all datasets. For random walk, we set the walk length to 30 and the window size to 5.
    \item \emph{GCN:} $d=64$ and $L=2$ for all datasets.
    \item \emph{GAT:} For LastFM, $d=64$, $n_h=4$, $L=3$, and $s=0.1$. For DBLP, $d=64$, $n_h=8$, $L=3$, and $s=0.05$. For IMDB, $d=64$, $n_h=4$, $L=5$, and $s=0.1$.
    \item \emph{SimpleHGN:} $d=64$, $d_e=32$, $n_h=2$, the edge residual $\beta=0$, and $s=0.01$ for all datasets. For DBLP, we set $L=3$. For LastFM,  $L=4$. For IMDB,  $L=6$.
    \item \emph{AutoAC:} We set $\lambda$ to 0.4 for all datasets, and $M$ to 8 for all datasets, which are consistent with the original paper.
    
\end{itemize}
